# Supplementary material for: Estimating influenza incidence using search query deceptiveness and generalized ridge regression
Source: arXiv:1901.03677 ancillary file (2019-01-11)
Supplement: Supplementary file 1 [file S4_Figures.pdf]

training: 3 seasons

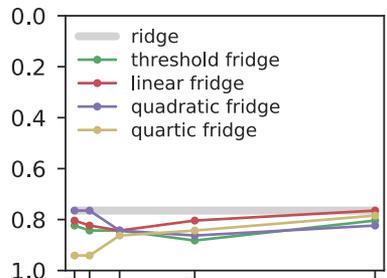2 seasons  
synthetic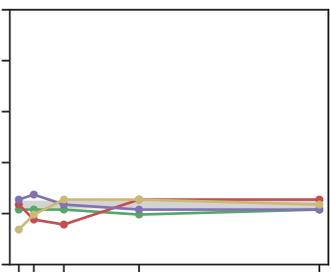

1 season

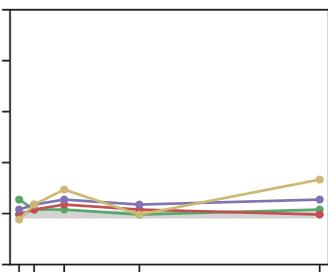

query strings

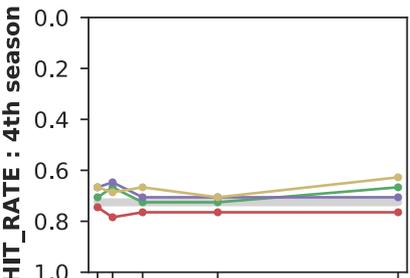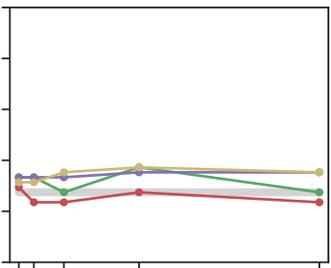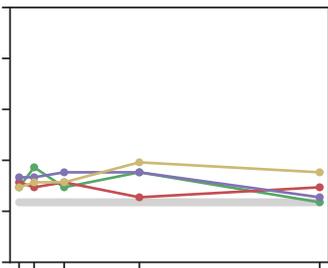

topics

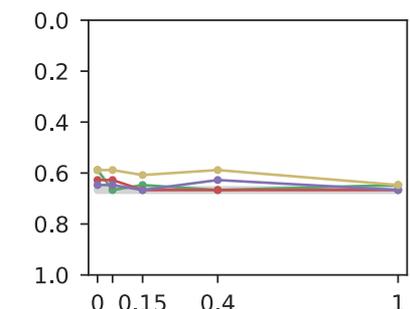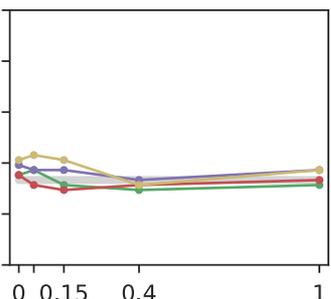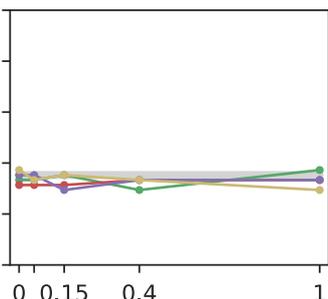

deceptiveness noise added

training: 3 seasons

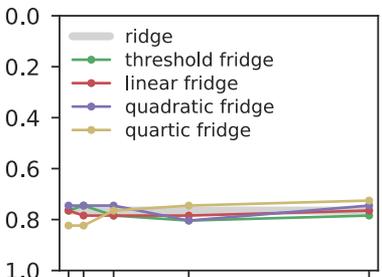2 seasons  
synthetic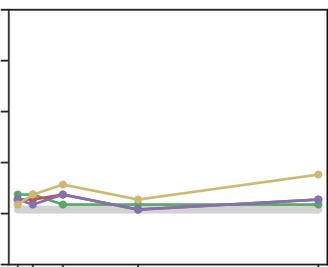

1 season

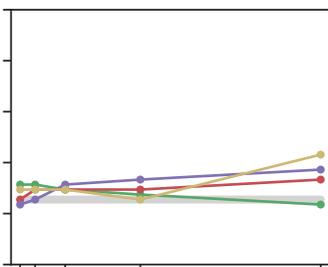

query strings

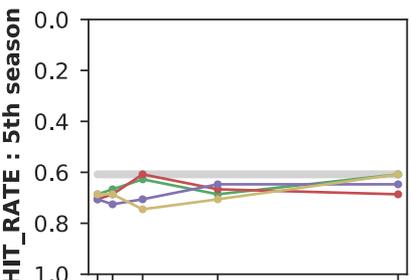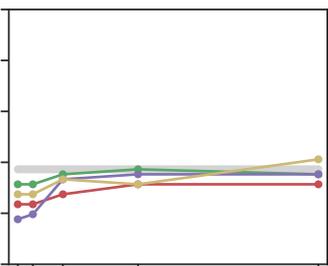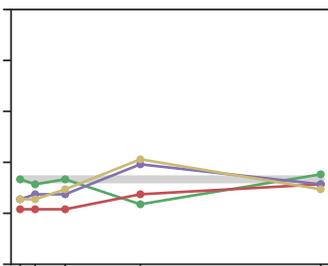

topics

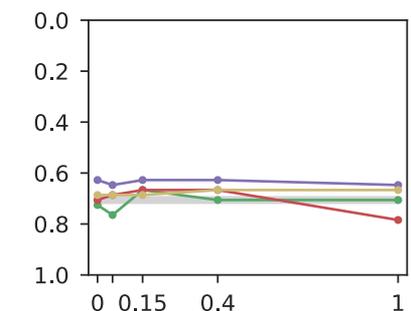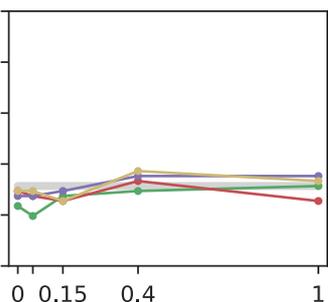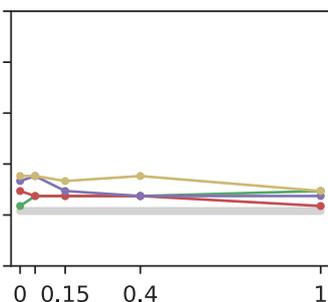

deceptive noise added

training: 3 seasons

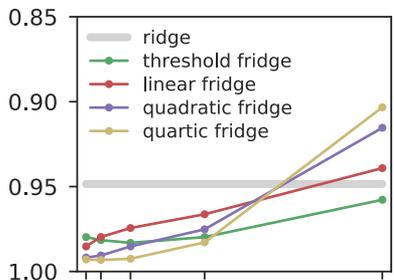2 seasons  
synthetic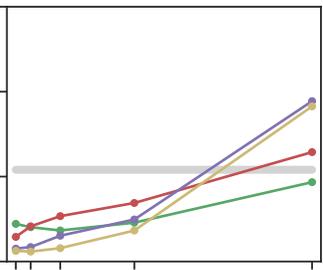

1 season

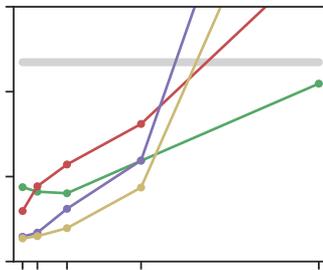

query strings

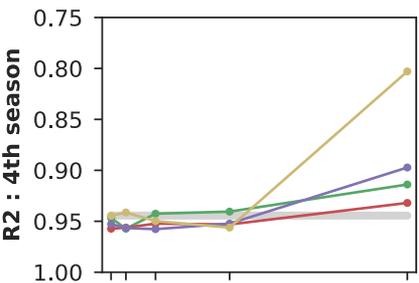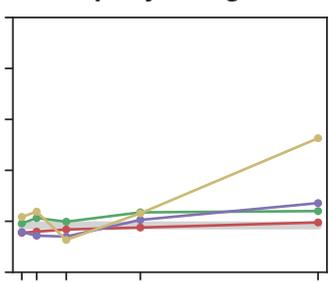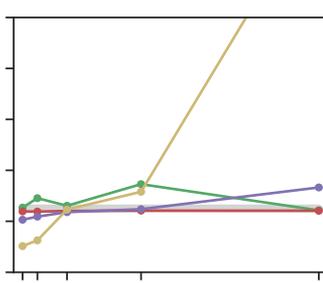

R2 : 4th season

topics

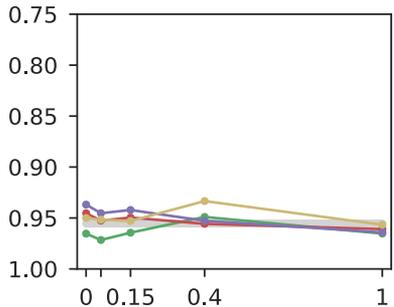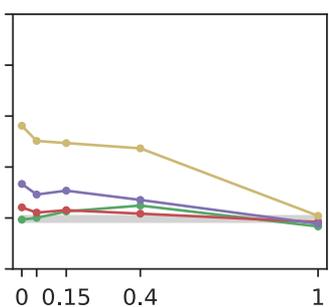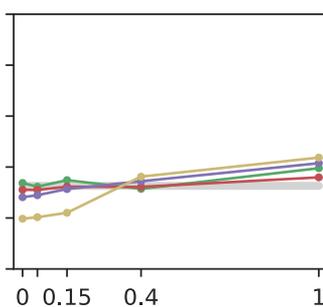

deceptiveness noise added

training: 3 seasons

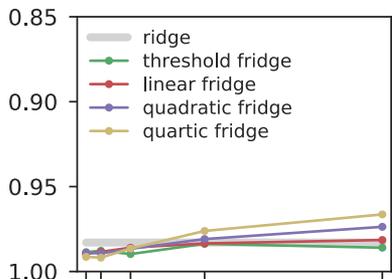2 seasons  
synthetic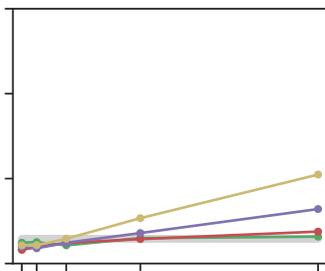

1 season

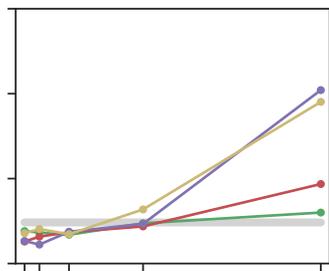

query strings

R2 : 5th season

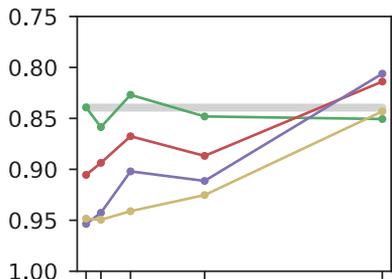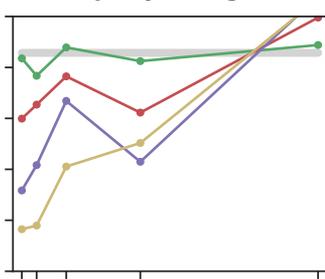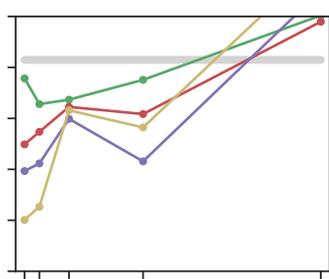

topics

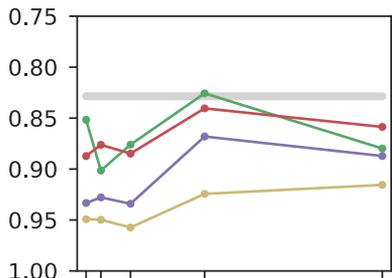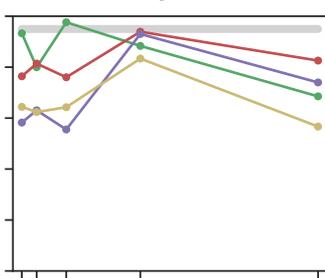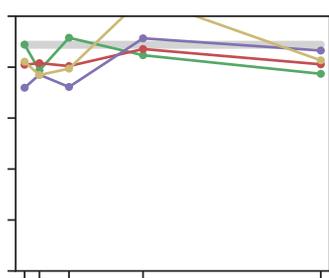

deceptiveness noise added

**training: 3 seasons****2 seasons  
synthetic****1 season**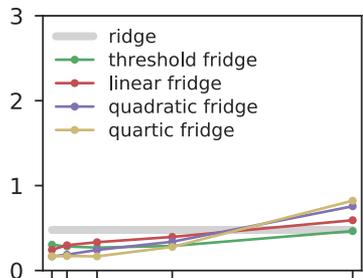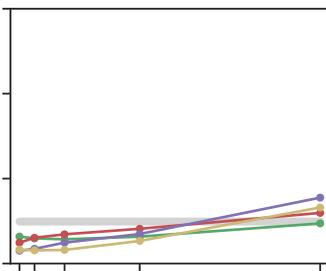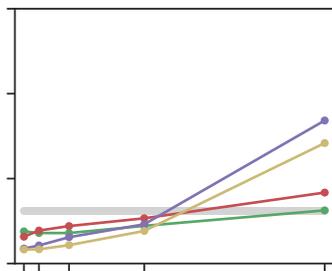**query strings****RMSE : 4th season**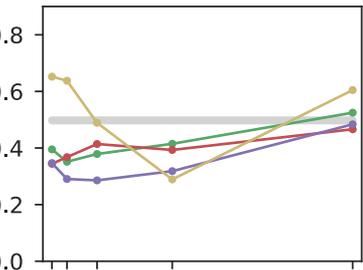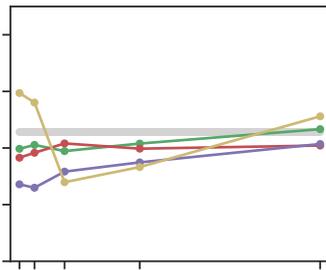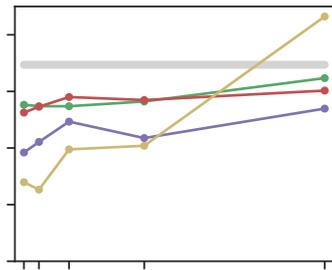**topics**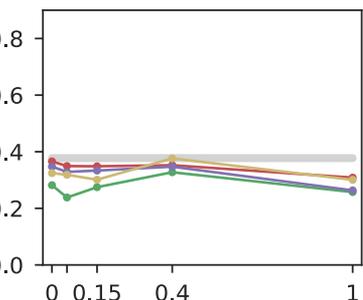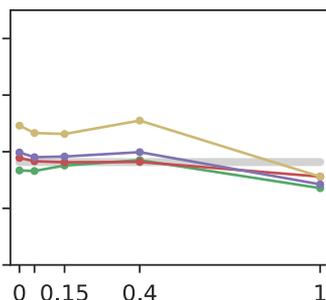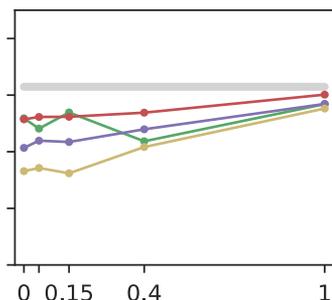**deceptiveness noise added**

training: 3 seasons

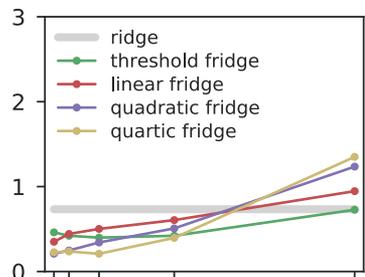2 seasons  
synthetic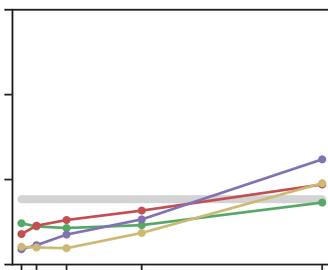

1 season

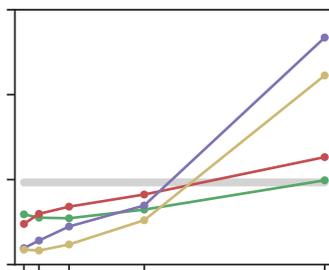

query strings

RMSE : 5th season

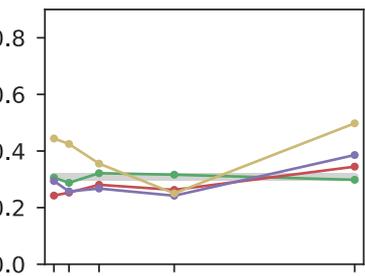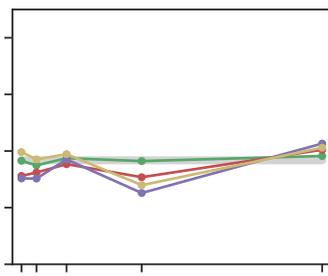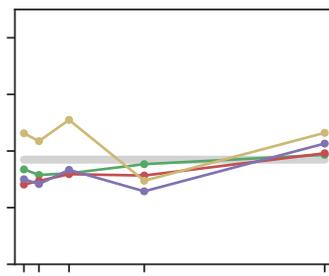

topics

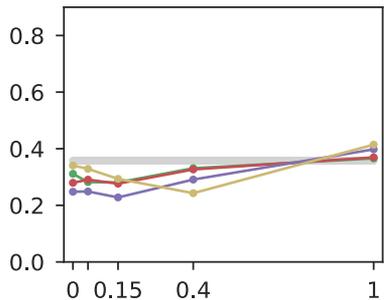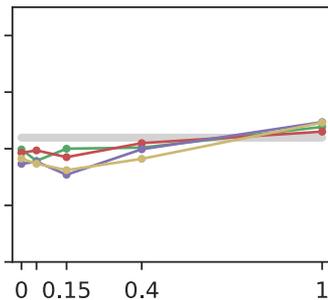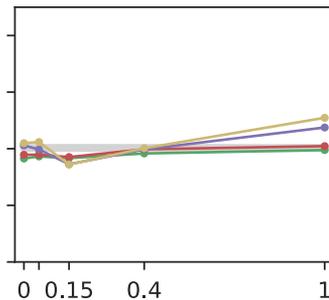

deceptiveness noise added
